# Supplementary material for: Molecular Dynamics Simulation Study of Nonconcatenated Ring Polymers in a Melt: II. Dynamics
Source: arXiv:1104.5655 ancillary file (2011-04-29)
Supplement: Supplementary file 1 [file ring_polymer_melts_dynamics_supplementary_material.pdf]

Supplementary Material

April 29, 2011

J. D. Halverson, W. Lee, G. S. Grest, A. Y. Grosberg and K. Kremer*, Molecular Dynamics Simulation Study of Nonconcatenated Ring Polymers in a Melt: II. Dynamics, Journal of Chemical Physics, DOI: 10.1063/1.3587138 (2011).

This document contains mean-square displacement data for the rings and linear systems as well as the various relaxation times of the rings. See Eqs. 2–4 of the article for the definitions of the various mean-square displacements. For the linear systems $g_1(t)$ and $g_2(t)$ were computed using the inner monomers.

*Corresponding author e-mail: kremer@mpip-mainz.mpg.de

Rings $N = 100$

| $t/\tau$ | $g_1(t)/\sigma^2$ | $g_2(t)/\sigma^2$ | $g_3(t)/\sigma^2$ |
|---|---|---|---|
| 0 | 0.0 | 0.0 | 0.0 |
| 1000 | 18.5 | 14.9 | 3.6 |
| 2000 | 25.8 | 19.5 | 6.3 |
| 3000 | 31.4 | 22.5 | 8.9 |
| 4000 | 36.1 | 24.7 | 11.5 |
| 5000 | 40.2 | 26.3 | 13.9 |
| 10000 | 56.7 | 30.8 | 25.9 |
| 15000 | 70.2 | 32.7 | 37.4 |
| 20000 | 82.7 | 33.5 | 49.2 |
| 25000 | 94.0 | 33.9 | 60.1 |
| 30000 | 105.5 | 33.9 | 71.6 |
| 35000 | 117.5 | 34.2 | 83.2 |
| 40000 | 129.2 | 34.3 | 94.9 |
| 45000 | 141.0 | 34.2 | 106.8 |
| 50000 | 152.4 | 34.2 | 118.2 |
| 55000 | 163.5 | 34.3 | 129.2 |
| 60000 | 175.4 | 34.4 | 141.1 |
| 70000 | 198.3 | 34.4 | 163.9 |
| 75000 | 209.7 | 34.3 | 175.4 |
| 85000 | 233.5 | 34.2 | 199.3 |
| 95000 | 256.5 | 34.2 | 222.3 |
| 110000 | 290.5 | 34.2 | 256.3 |
| 120000 | 313.7 | 34.3 | 279.4 |
| 135000 | 349.0 | 34.3 | 314.7 |
| 155000 | 396.1 | 34.2 | 361.8 |
| 170000 | 429.4 | 34.1 | 395.4 |
| 195000 | 486.3 | 34.3 | 452.0 |
| 215000 | 530.6 | 34.2 | 496.3 |
| 245000 | 599.1 | 34.1 | 565.0 |
| 275000 | 667.2 | 34.2 | 633.0 |
| 305000 | 738.4 | 34.2 | 704.2 |
| 345000 | 832.3 | 34.3 | 798.0 |
| 385000 | 923.0 | 34.0 | 889.0 |
| 435000 | 1035.0 | 34.3 | 1000.6 |
| 485000 | 1150.4 | 34.3 | 1116.1 |
| 545000 | 1290.3 | 34.3 | 1256.0 |
| 615000 | 1446.3 | 34.3 | 1412.1 |
| 690000 | 1615.6 | 34.3 | 1581.2 |
| 775000 | 1811.9 | 34.2 | 1777.7 |
| 870000 | 2021.7 | 34.3 | 1987.4 |
| 975000 | 2268.0 | 34.2 | 2233.8 |
| 1095000 | 2543.0 | 34.3 | 2508.7 |
| 1230000 | 2850.9 | 34.3 | 2816.6 |
| 1380000 | 3195.9 | 34.3 | 3161.7 |
| 1550000 | 3598.1 | 34.3 | 3563.8 |
| 1740000 | 4044.0 | 34.3 | 4009.7 |
| 1950000 | 4519.7 | 34.3 | 4485.4 |

| | | | |
|---|---|---|---|
| 2190000 | 5056.4 | 34.3 | 5022.1 |
| 2460000 | 5670.9 | 34.3 | 5636.7 |
| 2765000 | 6360.8 | 34.4 | 6326.5 |
| 3100000 | 7142.8 | 34.3 | 7108.5 |
| 3485000 | 8022.7 | 34.1 | 7988.5 |
| 3910000 | 9015.9 | 34.2 | 8981.7 |
| 4390000 | 10098.9 | 34.3 | 10064.6 |
| 4930000 | 11349.9 | 34.3 | 11315.7 |
| 5535000 | 12742.2 | 34.3 | 12708.0 |
| 6215000 | 14333.5 | 34.3 | 14299.2 |
| 6975000 | 16166.4 | 34.3 | 16132.1 |
| 7830000 | 18202.5 | 34.0 | 18168.5 |
| 8795000 | 20530.6 | 34.2 | 20496.3 |
| 9870000 | 23053.9 | 34.2 | 23019.8 |
| 11085000 | 26059.8 | 34.1 | 26025.7 |
| 12445000 | 29396.3 | 34.2 | 29362.1 |
| 13970000 | 32966.7 | 34.2 | 32932.5 |
| 15685000 | 36931.5 | 34.0 | 36897.5 |
| 17610000 | 42363.9 | 34.5 | 42329.4 |
| 19775000 | 46749.0 | 35.1 | 46713.9 |
| 19995000 | 47356.0 | 34.8 | 47321.2 |

Table 1: $g_i(t)$ for the rings with $N = 100$.

Rings $N = 200$

| $t/\tau$ | $g_1(t)/\sigma^2$ | $g_2(t)/\sigma^2$ | $g_3(t)/\sigma^2$ |
|---|---|---|---|
| 0 | 0.0 | 0.0 | 0.0 |
| 1000 | 18.0 | 16.0 | 2.0 |
| 2000 | 24.9 | 21.5 | 3.4 |
| 3000 | 29.8 | 25.2 | 4.6 |
| 4000 | 33.8 | 28.0 | 5.8 |
| 5000 | 37.2 | 30.4 | 6.9 |
| 10000 | 50.1 | 38.2 | 11.9 |
| 15000 | 59.7 | 43.1 | 16.6 |
| 20000 | 67.5 | 46.6 | 20.9 |
| 25000 | 74.4 | 49.3 | 25.1 |
| 30000 | 80.6 | 51.3 | 29.3 |
| 35000 | 86.2 | 52.9 | 33.4 |
| 40000 | 91.7 | 54.3 | 37.4 |
| 45000 | 97.0 | 55.4 | 41.6 |
| 50000 | 101.9 | 56.3 | 45.6 |
| 55000 | 106.9 | 57.1 | 49.7 |
| 60000 | 110.7 | 57.6 | 53.1 |
| 70000 | 120.0 | 58.8 | 61.2 |
| 75000 | 124.0 | 59.2 | 64.8 |
| 85000 | 132.1 | 59.6 | 72.5 |
| 95000 | 141.1 | 60.1 | 81.1 |
| 110000 | 153.2 | 60.4 | 92.8 |
| 120000 | 160.4 | 60.5 | 99.9 |
| 135000 | 172.3 | 60.8 | 111.5 |
| 155000 | 187.4 | 61.0 | 126.4 |
| 170000 | 200.0 | 61.1 | 138.9 |
| 195000 | 219.7 | 61.2 | 158.6 |
| 215000 | 237.0 | 61.2 | 175.8 |
| 245000 | 260.8 | 61.4 | 199.4 |
| 275000 | 283.6 | 61.5 | 222.2 |
| 305000 | 308.2 | 61.6 | 246.6 |
| 345000 | 337.7 | 61.6 | 276.1 |
| 385000 | 367.8 | 61.5 | 306.3 |
| 435000 | 407.5 | 61.7 | 345.8 |
| 485000 | 446.8 | 61.5 | 385.3 |
| 545000 | 491.6 | 61.4 | 430.2 |
| 615000 | 546.8 | 61.6 | 485.1 |
| 690000 | 605.3 | 61.3 | 543.9 |
| 775000 | 667.7 | 61.4 | 606.3 |
| 870000 | 743.5 | 61.5 | 682.0 |
| 975000 | 822.8 | 61.4 | 761.4 |
| 1095000 | 917.5 | 61.3 | 856.2 |
| 1230000 | 1022.5 | 61.6 | 960.9 |
| 1380000 | 1136.6 | 61.7 | 1075.0 |
| 1550000 | 1269.4 | 61.4 | 1208.1 |
| 1740000 | 1417.8 | 61.3 | 1356.5 |
| 1950000 | 1580.9 | 61.4 | 1519.5 |

| | | | |
|---|---|---|---|
| 2190000 | 1770.4 | 61.6 | 1708.8 |
| 2460000 | 1984.1 | 61.5 | 1922.6 |
| 2765000 | 2231.5 | 61.4 | 2170.0 |
| 3100000 | 2504.5 | 61.4 | 2443.1 |
| 3485000 | 2809.8 | 61.5 | 2748.3 |
| 3910000 | 3148.7 | 61.3 | 3087.4 |
| 4390000 | 3530.6 | 61.6 | 3469.0 |
| 4930000 | 3948.7 | 61.4 | 3887.3 |
| 5535000 | 4413.9 | 61.3 | 4352.7 |
| 6215000 | 4927.4 | 61.8 | 4865.6 |
| 6975000 | 5511.2 | 61.6 | 5449.5 |
| 7830000 | 6166.6 | 61.5 | 6105.1 |
| 8795000 | 6933.7 | 61.4 | 6872.2 |
| 9870000 | 7771.1 | 61.5 | 7709.6 |
| 11085000 | 8701.6 | 60.9 | 8640.7 |
| 12445000 | 9767.7 | 61.6 | 9706.1 |
| 13970000 | 11121.9 | 61.4 | 11060.5 |
| 15685000 | 12658.8 | 61.3 | 12597.5 |
| 17610000 | 14374.2 | 61.4 | 14312.8 |
| 19775000 | 16369.0 | 60.8 | 16308.2 |
| 19995000 | 16465.2 | 61.4 | 16403.8 |

Table 2: $g_i(t)$ for the rings with $N = 200$.

Rings $N = 400$

| $t/\tau$ | $g_1(t)/\sigma^2$ | $g_2(t)/\sigma^2$ | $g_3(t)/\sigma^2$ |
|---|---|---|---|
| 0 | 0.0 | 0.0 | 0.0 |
| 1000 | 17.8 | 16.6 | 1.1 |
| 2000 | 24.5 | 22.5 | 1.9 |
| 3000 | 29.2 | 26.6 | 2.6 |
| 4000 | 33.0 | 29.8 | 3.3 |
| 5000 | 36.3 | 32.4 | 3.8 |
| 6000 | 39.0 | 34.7 | 4.4 |
| 7000 | 41.6 | 36.7 | 4.9 |
| 8000 | 43.8 | 38.5 | 5.3 |
| 9000 | 45.9 | 40.1 | 5.8 |
| 10000 | 47.9 | 41.6 | 6.3 |
| 20000 | 62.9 | 52.3 | 10.6 |
| 30000 | 73.7 | 59.3 | 14.3 |
| 40000 | 81.8 | 64.3 | 17.5 |
| 50000 | 89.0 | 68.5 | 20.5 |
| 60000 | 95.1 | 71.7 | 23.4 |
| 70000 | 100.6 | 74.4 | 26.2 |
| 80000 | 105.9 | 77.0 | 28.9 |
| 90000 | 110.8 | 79.2 | 31.6 |
| 100000 | 115.2 | 81.2 | 34.0 |
| 110000 | 119.2 | 82.8 | 36.4 |
| 120000 | 123.1 | 84.3 | 38.7 |
| 140000 | 130.4 | 86.8 | 43.6 |
| 150000 | 134.3 | 88.1 | 46.1 |
| 170000 | 141.0 | 90.3 | 50.7 |
| 190000 | 147.9 | 92.0 | 55.8 |
| 220000 | 156.8 | 93.9 | 62.9 |
| 240000 | 162.4 | 95.2 | 67.2 |
| 270000 | 170.4 | 96.9 | 73.5 |
| 310000 | 181.0 | 98.5 | 82.5 |
| 340000 | 188.4 | 99.2 | 89.2 |
| 390000 | 201.3 | 100.9 | 100.4 |
| 430000 | 211.2 | 101.9 | 109.3 |
| 490000 | 225.7 | 102.9 | 122.7 |
| 550000 | 238.5 | 103.7 | 134.8 |
| 610000 | 252.2 | 103.9 | 148.2 |
| 690000 | 270.1 | 104.5 | 165.6 |
| 770000 | 286.2 | 104.7 | 181.5 |
| 870000 | 309.2 | 105.2 | 204.0 |
| 970000 | 329.3 | 105.2 | 224.1 |
| 1090000 | 355.7 | 105.8 | 249.9 |
| 1230000 | 385.2 | 105.4 | 279.8 |
| 1380000 | 416.3 | 105.3 | 311.0 |
| 1550000 | 452.4 | 106.0 | 346.4 |
| 1740000 | 493.6 | 105.7 | 387.9 |
| 1950000 | 540.5 | 106.0 | 434.5 |
| 2190000 | 593.6 | 105.9 | 487.6 |

| | | | |
|---|---|---|---|
| 2460000 | 651.2 | 105.6 | 545.5 |
| 2760000 | 717.1 | 105.7 | 611.4 |
| 3100000 | 790.1 | 105.7 | 684.3 |
| 3480000 | 871.2 | 106.2 | 765.0 |
| 3910000 | 961.3 | 106.0 | 855.3 |
| 4390000 | 1068.4 | 105.7 | 962.7 |
| 4930000 | 1186.0 | 105.8 | 1080.3 |
| 5530000 | 1319.7 | 105.6 | 1214.1 |
| 6210000 | 1474.2 | 105.3 | 1368.9 |
| 6980000 | 1640.1 | 105.2 | 1534.9 |
| 7830000 | 1815.5 | 105.5 | 1710.0 |
| 8790000 | 2022.1 | 105.8 | 1916.3 |
| 9870000 | 2255.8 | 105.9 | 2149.8 |
| 11080000 | 2513.4 | 105.7 | 2407.7 |
| 12440000 | 2791.1 | 106.0 | 2685.2 |
| 13970000 | 3083.8 | 105.6 | 2978.2 |
| 15690000 | 3395.8 | 106.5 | 3289.3 |
| 17610000 | 3774.8 | 106.2 | 3668.5 |
| 19770000 | 4162.0 | 103.5 | 4058.5 |
| 19990000 | 4211.9 | 105.4 | 4106.5 |

Table 3: $g_i(t)$ for the rings with $N = 400$.

Rings $N = 800$

| $t/\tau$ | $g_1(t)/\sigma^2$ | $g_2(t)/\sigma^2$ | $g_3(t)/\sigma^2$ |
|---|---|---|---|
| 0 | 0.0 | 0.0 | 0.0 |
| 1000 | 17.7 | 17.0 | 0.6 |
| 2000 | 24.2 | 23.1 | 1.1 |
| 3000 | 28.9 | 27.4 | 1.5 |
| 4000 | 32.5 | 30.7 | 1.8 |
| 5000 | 35.6 | 33.5 | 2.2 |
| 6000 | 38.4 | 35.9 | 2.5 |
| 7000 | 40.8 | 38.1 | 2.7 |
| 8000 | 43.0 | 40.0 | 3.0 |
| 9000 | 45.0 | 41.8 | 3.2 |
| 10000 | 46.9 | 43.4 | 3.5 |
| 20000 | 60.9 | 55.2 | 5.7 |
| 30000 | 70.6 | 63.0 | 7.6 |
| 40000 | 78.0 | 68.8 | 9.1 |
| 50000 | 84.2 | 73.6 | 10.6 |
| 60000 | 89.7 | 77.7 | 12.0 |
| 70000 | 94.7 | 81.3 | 13.3 |
| 80000 | 99.0 | 84.5 | 14.5 |
| 90000 | 102.9 | 87.2 | 15.7 |
| 100000 | 106.6 | 89.7 | 16.9 |
| 110000 | 110.0 | 92.2 | 17.8 |
| 120000 | 113.2 | 94.3 | 18.8 |
| 140000 | 119.1 | 98.2 | 21.0 |
| 150000 | 121.7 | 99.8 | 21.8 |
| 170000 | 126.8 | 103.2 | 23.6 |
| 190000 | 131.4 | 106.0 | 25.4 |
| 220000 | 137.7 | 109.8 | 27.8 |
| 240000 | 141.7 | 112.0 | 29.7 |
| 270000 | 147.0 | 115.1 | 31.9 |
| 310000 | 153.2 | 118.6 | 34.7 |
| 340000 | 158.1 | 121.0 | 37.1 |
| 390000 | 164.9 | 124.7 | 40.2 |
| 430000 | 169.9 | 127.1 | 42.7 |
| 490000 | 177.2 | 130.5 | 46.7 |
| 550000 | 184.6 | 133.4 | 51.2 |
| 610000 | 190.8 | 136.1 | 54.7 |
| 690000 | 198.9 | 139.2 | 59.7 |
| 770000 | 206.4 | 142.1 | 64.3 |
| 870000 | 214.6 | 144.9 | 69.7 |
| 970000 | 223.2 | 147.5 | 75.7 |
| 1090000 | 232.8 | 150.2 | 82.6 |
| 1230000 | 243.0 | 152.9 | 90.1 |
| 1380000 | 253.4 | 155.6 | 97.8 |
| 1550000 | 264.8 | 157.9 | 106.9 |
| 1740000 | 276.6 | 159.8 | 116.8 |
| 1950000 | 289.3 | 161.7 | 127.6 |
| 2190000 | 303.2 | 163.7 | 139.5 |

| | | | |
|---|---|---|---|
| 2460000 | 318.3 | 165.4 | 152.9 |
| 2760000 | 334.8 | 167.1 | 167.7 |
| 3100000 | 353.5 | 168.8 | 184.8 |
| 3480000 | 372.8 | 170.3 | 202.4 |
| 3910000 | 395.0 | 171.5 | 223.5 |
| 4390000 | 417.5 | 172.4 | 245.0 |
| 4930000 | 441.9 | 173.1 | 268.8 |
| 5530000 | 469.2 | 173.8 | 295.3 |
| 6210000 | 497.5 | 174.5 | 323.0 |
| 6980000 | 532.7 | 175.1 | 357.7 |
| 7830000 | 569.5 | 175.1 | 394.3 |
| 8790000 | 608.6 | 175.0 | 433.5 |
| 9870000 | 651.7 | 175.6 | 476.0 |
| 11080000 | 697.1 | 176.5 | 520.6 |
| 12440000 | 746.2 | 176.2 | 569.9 |
| 13970000 | 807.4 | 176.9 | 630.5 |
| 15690000 | 876.4 | 175.8 | 700.6 |
| 17610000 | 956.6 | 176.2 | 780.4 |
| 19690000 | 1056.6 | 180.2 | 876.5 |

Table 4: $g_i(t)$ for the rings with $N = 800$.

| Rings $N = 1600$ | | | |
|---|---|---|---|
| $t/\tau$ | $g_1(t)/\sigma^2$ | $g_2(t)/\sigma^2$ | $g_3(t)/\sigma^2$ |
| 0 | 0.0 | 0.0 | 0.0 |
| 1000 | 17.6 | 17.3 | 0.4 |
| 2000 | 24.2 | 23.5 | 0.6 |
| 3000 | 28.8 | 27.9 | 0.9 |
| 4000 | 32.5 | 31.4 | 1.1 |
| 5000 | 35.6 | 34.3 | 1.3 |
| 6000 | 38.3 | 36.8 | 1.4 |
| 7000 | 40.7 | 39.1 | 1.6 |
| 8000 | 42.9 | 41.1 | 1.8 |
| 9000 | 44.9 | 42.9 | 1.9 |
| 10000 | 46.8 | 44.7 | 2.1 |
| 20000 | 60.8 | 57.4 | 3.3 |
| 30000 | 70.3 | 65.9 | 4.4 |
| 40000 | 77.6 | 72.3 | 5.3 |
| 50000 | 83.9 | 77.8 | 6.1 |
| 60000 | 89.1 | 82.2 | 6.9 |
| 70000 | 93.9 | 86.2 | 7.6 |
| 80000 | 98.0 | 89.8 | 8.2 |
| 90000 | 101.8 | 93.0 | 8.8 |
| 100000 | 105.3 | 95.9 | 9.4 |
| 110000 | 108.7 | 98.7 | 10.0 |
| 120000 | 111.8 | 101.3 | 10.5 |
| 140000 | 117.2 | 105.7 | 11.5 |
| 150000 | 119.9 | 107.8 | 12.0 |
| 170000 | 124.7 | 111.6 | 13.1 |
| 190000 | 129.0 | 115.2 | 13.9 |
| 220000 | 135.0 | 119.8 | 15.2 |
| 240000 | 138.5 | 122.5 | 16.0 |
| 270000 | 143.7 | 126.5 | 17.2 |
| 310000 | 149.8 | 131.2 | 18.6 |
| 340000 | 153.5 | 134.1 | 19.4 |
| 390000 | 160.1 | 139.0 | 21.1 |
| 430000 | 164.9 | 142.5 | 22.4 |
| 490000 | 171.3 | 147.2 | 24.1 |
| 550000 | 177.2 | 151.4 | 25.8 |
| 610000 | 182.6 | 155.2 | 27.4 |
| 690000 | 189.0 | 159.6 | 29.4 |
| 770000 | 194.7 | 163.4 | 31.3 |
| 870000 | 201.6 | 167.9 | 33.8 |
| 970000 | 207.7 | 171.8 | 35.9 |
| 1090000 | 215.3 | 176.6 | 38.6 |
| 1230000 | 223.1 | 181.4 | 41.7 |
| 1380000 | 230.9 | 186.0 | 44.9 |
| 1550000 | 239.1 | 190.9 | 48.2 |
| 1740000 | 247.4 | 195.5 | 52.0 |
| 1950000 | 255.8 | 200.2 | 55.6 |
| 2190000 | 264.8 | 204.8 | 60.0 |

| | | | |
|---|---|---|---|
| 2460000 | 274.5 | 209.6 | 64.9 |
| 2760000 | 284.2 | 214.4 | 69.8 |
| 3100000 | 293.8 | 219.1 | 74.7 |
| 3480000 | 304.7 | 224.0 | 80.7 |
| 3910000 | 315.0 | 228.5 | 86.5 |
| 4390000 | 326.0 | 233.3 | 92.7 |
| 4930000 | 337.2 | 237.9 | 99.3 |
| 5530000 | 348.7 | 241.9 | 106.8 |
| 6210000 | 361.3 | 245.8 | 115.4 |
| 6980000 | 376.2 | 250.2 | 126.0 |
| 7830000 | 391.3 | 255.3 | 136.1 |
| 8790000 | 408.7 | 260.0 | 148.7 |
| 9870000 | 427.2 | 264.1 | 163.1 |
| 11080000 | 446.9 | 268.9 | 178.0 |
| 12440000 | 464.5 | 271.5 | 193.0 |
| 13970000 | 485.1 | 274.6 | 210.4 |
| 15690000 | 507.3 | 278.5 | 228.7 |
| 17610000 | 530.6 | 281.4 | 249.1 |
| 19770000 | 548.6 | 279.9 | 268.7 |
| 19790000 | 545.1 | 276.5 | 268.6 |

Table 5: $g_i(t)$ for the rings with $N = 1600$.

Linear $N = 100$

| $t/\tau$ | $g_1(t)/\sigma^2$ | $g_2(t)/\sigma^2$ | $g_3(t)/\sigma^2$ |
|---|---|---|---|
| 1200 | 17.7 | 14.5 | 3.3 |
| 2400 | 23.3 | 18.5 | 5.3 |
| 3600 | 27.1 | 21.2 | 7.0 |
| 4800 | 30.1 | 23.3 | 8.5 |
| 6000 | 32.7 | 25.0 | 10.0 |
| 7200 | 34.9 | 26.5 | 11.4 |
| 8400 | 36.9 | 27.7 | 12.7 |
| 9600 | 38.8 | 28.9 | 14.0 |
| 10800 | 40.5 | 29.9 | 15.2 |
| 12000 | 42.1 | 30.8 | 16.5 |
| 14400 | 45.1 | 32.4 | 18.9 |
| 18000 | 49.4 | 34.3 | 22.4 |
| 21600 | 53.3 | 35.8 | 25.9 |
| 25200 | 57.0 | 37.0 | 29.2 |
| 28800 | 60.6 | 37.9 | 32.5 |
| 32400 | 64.0 | 38.6 | 35.7 |
| 36000 | 67.2 | 39.1 | 38.9 |
| 39600 | 70.5 | 39.5 | 42.0 |
| 43200 | 73.8 | 39.8 | 45.2 |
| 46800 | 77.1 | 40.1 | 48.4 |
| 50400 | 80.4 | 40.3 | 51.6 |
| 54000 | 83.6 | 40.5 | 54.8 |
| 57600 | 86.8 | 40.6 | 58.0 |
| 72000 | 99.6 | 40.9 | 70.6 |
| 84000 | 110.3 | 41.1 | 81.3 |
| 96000 | 121.2 | 41.1 | 92.4 |
| 108000 | 132.0 | 41.2 | 103.3 |
| 120000 | 142.6 | 41.5 | 113.8 |
| 132000 | 153.0 | 41.5 | 124.2 |
| 144000 | 163.1 | 41.5 | 134.3 |
| 156000 | 174.0 | 41.6 | 144.8 |
| 168000 | 184.8 | 41.6 | 155.5 |
| 180000 | 195.5 | 41.4 | 166.4 |
| 192000 | 206.3 | 41.4 | 177.3 |
| 204000 | 217.2 | 41.4 | 188.5 |
| 216000 | 228.7 | 41.5 | 200.1 |
| 228000 | 240.7 | 41.4 | 211.8 |
| 240000 | 252.2 | 41.4 | 223.2 |
| 252000 | 263.2 | 41.5 | 234.4 |
| 264000 | 274.5 | 41.6 | 245.7 |
| 276000 | 285.4 | 41.7 | 257.0 |
| 288000 | 296.6 | 41.5 | 268.1 |
| 300000 | 307.8 | 41.6 | 278.7 |
| 312000 | 318.5 | 41.4 | 289.0 |
| 324000 | 328.8 | 41.2 | 299.3 |
| 336000 | 339.1 | 41.3 | 309.7 |
| 360000 | 358.5 | 41.4 | 329.0 |

| | | | |
|---|---|---|---|
| 396000 | 386.3 | 41.6 | 356.7 |
| 432000 | 417.4 | 41.4 | 387.9 |
| 468000 | 451.5 | 41.3 | 422.0 |
| 504000 | 485.3 | 41.3 | 456.5 |
| 540000 | 521.0 | 41.4 | 491.6 |

Table 6: $g_i(t)$ for the linear with $N = 100$.

| Linear $N = 200$ | | | |
|---|---|---|---|
| $t/\tau$ | $g_1(t)/\sigma^2$ | $g_2(t)/\sigma^2$ | $g_3(t)/\sigma^2$ |
| 1200.0 | 17.1 | 15.5 | 1.6 |
| 2400.0 | 22.1 | 19.7 | 2.4 |
| 3600.0 | 25.5 | 22.5 | 3.1 |
| 4800.0 | 28.0 | 24.6 | 3.7 |
| 6000.0 | 30.1 | 26.3 | 4.2 |
| 7200.0 | 31.8 | 27.8 | 4.7 |
| 8400.0 | 33.4 | 29.1 | 5.1 |
| 9600.0 | 34.8 | 30.3 | 5.5 |
| 10800.0 | 36.1 | 31.4 | 5.9 |
| 12000.0 | 37.3 | 32.3 | 6.3 |
| 14400.0 | 39.4 | 34.1 | 7.1 |
| 18000.0 | 42.1 | 36.4 | 8.1 |
| 21600.0 | 44.5 | 38.5 | 9.0 |
| 25200.0 | 46.7 | 40.3 | 10.0 |
| 28800.0 | 48.6 | 41.9 | 10.9 |
| 32400.0 | 50.4 | 43.5 | 11.7 |
| 36000.0 | 52.1 | 44.9 | 12.6 |
| 43200.0 | 55.2 | 47.4 | 14.2 |
| 46800.0 | 56.6 | 48.6 | 15.0 |
| 54000.0 | 59.3 | 50.8 | 16.5 |
| 57600.0 | 60.6 | 51.9 | 17.2 |
| 72000.0 | 65.5 | 55.6 | 20.1 |
| 84000.0 | 69.0 | 58.2 | 22.5 |
| 96000.0 | 72.2 | 60.4 | 24.9 |
| 108000.0 | 75.2 | 62.3 | 27.3 |
| 120000.0 | 78.4 | 64.3 | 29.5 |
| 132000.0 | 81.2 | 66.0 | 31.8 |
| 156000.0 | 86.8 | 69.2 | 36.0 |
| 168000.0 | 89.4 | 70.5 | 38.1 |
| 192000.0 | 94.5 | 73.0 | 42.3 |
| 216000.0 | 99.5 | 75.2 | 46.7 |
| 240000.0 | 104.6 | 76.9 | 51.0 |
| 276000.0 | 111.2 | 78.7 | 57.1 |
| 300000.0 | 115.3 | 79.7 | 61.2 |
| 336000.0 | 121.5 | 81.3 | 67.3 |
| 396000.0 | 132.4 | 82.4 | 77.6 |
| 432000.0 | 139.1 | 83.3 | 83.7 |
| 504000.0 | 151.9 | 84.3 | 96.0 |
| 540000.0 | 158.4 | 84.7 | 101.8 |
| 612000.0 | 170.8 | 85.3 | 113.4 |
| 684000.0 | 183.0 | 86.8 | 124.8 |
| 792000.0 | 200.2 | 87.3 | 141.2 |
| 864000.0 | 211.8 | 87.1 | 152.3 |
| 972000.0 | 229.3 | 88.2 | 169.8 |
| 1080000.0 | 247.2 | 89.1 | 187.4 |
| 1188000.0 | 263.5 | 88.4 | 204.9 |

Table 7: $g_i(t)$ for the linear with $N = 200$.

| Linear $N = 400$ | | | |
|---|---|---|---|
| $t/\tau$ | $g_1(t)/\sigma^2$ | $g_2(t)/\sigma^2$ | $g_3(t)/\sigma^2$ |
| 1200 | 16.9 | 16.0 | 0.8 |
| 2400 | 21.7 | 20.4 | 1.3 |
| 3600 | 24.9 | 23.3 | 1.6 |
| 4800 | 27.3 | 25.4 | 1.8 |
| 6000 | 29.2 | 27.2 | 2.1 |
| 7200 | 30.8 | 28.7 | 2.3 |
| 8400 | 32.3 | 30.0 | 2.4 |
| 9600 | 33.5 | 31.1 | 2.6 |
| 10800 | 34.7 | 32.1 | 2.8 |
| 12000 | 35.7 | 33.1 | 2.9 |
| 14400 | 37.6 | 34.7 | 3.2 |
| 18000 | 39.9 | 36.8 | 3.6 |
| 21600 | 42.0 | 38.7 | 4.0 |
| 25200 | 43.8 | 40.3 | 4.3 |
| 28800 | 45.5 | 41.8 | 4.6 |
| 32400 | 46.9 | 43.1 | 4.9 |
| 36000 | 48.3 | 44.3 | 5.2 |
| 43200 | 50.8 | 46.6 | 5.8 |
| 46800 | 51.9 | 47.5 | 6.1 |
| 54000 | 54.0 | 49.4 | 6.6 |
| 57600 | 55.0 | 50.3 | 6.8 |
| 72000 | 58.3 | 53.3 | 7.8 |
| 84000 | 60.9 | 55.8 | 8.6 |
| 96000 | 63.1 | 57.7 | 9.3 |
| 108000 | 65.2 | 59.6 | 9.9 |
| 120000 | 67.2 | 61.5 | 10.6 |
| 132000 | 68.9 | 63.1 | 11.2 |
| 156000 | 72.2 | 66.4 | 12.4 |
| 168000 | 73.7 | 67.8 | 13.0 |
| 192000 | 76.5 | 70.5 | 14.2 |
| 216000 | 79.3 | 73.0 | 15.3 |
| 240000 | 82.0 | 75.5 | 16.4 |
| 264000 | 84.4 | 77.9 | 17.4 |
| 300000 | 87.8 | 81.2 | 18.9 |
| 336000 | 91.1 | 84.3 | 20.4 |
| 396000 | 96.1 | 89.2 | 22.8 |
| 432000 | 98.8 | 91.8 | 24.2 |
| 468000 | 101.4 | 94.4 | 25.7 |
| 540000 | 106.2 | 98.9 | 28.5 |
| 612000 | 110.7 | 102.9 | 31.2 |
| 684000 | 115.2 | 107.1 | 33.8 |
| 756000 | 120.0 | 111.1 | 36.5 |
| 864000 | 126.7 | 116.8 | 40.2 |
| 972000 | 132.3 | 121.9 | 43.9 |
| 1.08E6 | 136.9 | 125.7 | 47.5 |
| 1.224E6 | 143.5 | 130.6 | 52.4 |
| 1.368E6 | 149.9 | 135.4 | 57.2 |

| | | | |
|---|---|---|---|
| 1.548E6 | 158.1 | 141.0 | 62.8 |
| 1.728E6 | 166.3 | 146.1 | 68.3 |
| 1.944E6 | 175.4 | 151.3 | 74.6 |
| 2.16E6 | 182.6 | 155.5 | 81.0 |
| 2.448E6 | 191.8 | 159.1 | 89.3 |
| 2.736E6 | 199.3 | 161.0 | 97.5 |
| 3.06E6 | 209.6 | 163.6 | 106.8 |
| 3.456E6 | 222.7 | 167.3 | 117.9 |
| 3.888E6 | 236.1 | 171.1 | 130.0 |
| 4.356E6 | 247.4 | 173.8 | 142.9 |
| 4.896E6 | 265.0 | 175.9 | 158.9 |
| 5.472E6 | 280.0 | 176.1 | 174.4 |
| 6.156E6 | 302.7 | 176.7 | 194.7 |
| 6.912E6 | 324.4 | 177.6 | 212.9 |
| 7.776E6 | 348.4 | 176.8 | 234.0 |
| 8.748E6 | 378.3 | 173.4 | 263.4 |
| 9.792E6 | 413.7 | 175.0 | 299.2 |
| 1.1016E7 | 451.2 | 170.6 | 336.8 |
| 1.1988E7 | 473.4 | 170.7 | 360.8 |

Table 8: $g_i(t)$ for the linear with $N = 400$.

Linear $N = 800$

| $t/\tau$ | $g_1(t)/\sigma^2$ | $g_2(t)/\sigma^2$ | $g_3(t)/\sigma^2$ |
|---|---|---|---|
| 1200 | 16.7 | 16.2 | 0.5 |
| 2400 | 21.6 | 20.8 | 0.7 |
| 3600 | 24.6 | 23.7 | 0.8 |
| 4800 | 26.9 | 25.9 | 1.0 |
| 6000 | 28.8 | 27.7 | 1.1 |
| 7200 | 30.4 | 29.2 | 1.2 |
| 8400 | 31.8 | 30.5 | 1.3 |
| 9600 | 32.9 | 31.6 | 1.3 |
| 10800 | 34.0 | 32.6 | 1.4 |
| 12000 | 35.1 | 33.6 | 1.5 |
| 14400 | 36.8 | 35.2 | 1.6 |
| 18000 | 39.0 | 37.3 | 1.7 |
| 21600 | 41.1 | 39.3 | 1.9 |
| 25200 | 42.7 | 40.8 | 2.0 |
| 28800 | 44.2 | 42.2 | 2.1 |
| 32400 | 45.6 | 43.5 | 2.3 |
| 36000 | 46.8 | 44.7 | 2.4 |
| 43200 | 49.1 | 46.7 | 2.6 |
| 46800 | 50.2 | 47.8 | 2.7 |
| 54000 | 52.1 | 49.5 | 2.9 |
| 57600 | 52.9 | 50.3 | 2.9 |
| 72000 | 56.1 | 53.3 | 3.3 |
| 84000 | 58.2 | 55.4 | 3.5 |
| 96000 | 60.3 | 57.3 | 3.8 |
| 108000 | 62.4 | 59.2 | 4.0 |
| 120000 | 64.0 | 60.8 | 4.3 |
| 132000 | 65.7 | 62.4 | 4.5 |
| 156000 | 68.6 | 65.1 | 4.9 |
| 168000 | 69.9 | 66.3 | 5.1 |
| 192000 | 72.4 | 68.6 | 5.5 |
| 216000 | 74.6 | 70.7 | 5.9 |
| 240000 | 76.8 | 72.9 | 6.2 |
| 264000 | 78.8 | 74.8 | 6.6 |
| 300000 | 81.6 | 77.5 | 7.1 |
| 336000 | 84.2 | 80.0 | 7.5 |
| 396000 | 88.3 | 83.9 | 8.3 |
| 432000 | 90.5 | 86.0 | 8.8 |
| 468000 | 92.8 | 88.4 | 9.2 |
| 540000 | 96.8 | 92.2 | 10.1 |
| 612000 | 100.3 | 95.5 | 10.9 |
| 684000 | 103.8 | 98.9 | 11.7 |
| 756000 | 107.1 | 102.2 | 12.5 |
| 864000 | 111.7 | 106.4 | 13.6 |
| 972000 | 115.8 | 110.5 | 14.6 |
| 1.08E6 | 119.1 | 113.7 | 15.6 |
| 1.224E6 | 124.0 | 118.3 | 17.0 |
| 1.368E6 | 127.9 | 122.2 | 18.3 |

| | | | |
|---|---|---|---|
| 1.548E6 | 132.8 | 127.3 | 19.9 |
| 1.728E6 | 137.5 | 132.0 | 21.4 |
| 1.944E6 | 143.8 | 137.7 | 23.1 |
| 2.16E6 | 150.0 | 143.2 | 24.7 |
| 2.448E6 | 157.1 | 150.3 | 27.0 |
| 2.736E6 | 163.1 | 156.8 | 29.4 |
| 3.06E6 | 169.1 | 162.2 | 32.0 |
| 3.456E6 | 175.5 | 167.3 | 35.4 |
| 3.888E6 | 182.7 | 173.4 | 38.9 |
| 4.356E6 | 190.1 | 180.6 | 42.3 |
| 4.896E6 | 195.7 | 186.2 | 46.4 |
| 5.472E6 | 203.7 | 193.8 | 50.2 |
| 6.156E6 | 211.7 | 201.7 | 54.4 |
| 6.912E6 | 220.4 | 209.7 | 59.4 |
| 7.776E6 | 228.8 | 215.8 | 65.0 |
| 8.748E6 | 238.9 | 223.0 | 70.7 |
| 9.792E6 | 245.8 | 226.6 | 75.7 |
| 1.1016E7 | 254.5 | 232.2 | 84.6 |
| 1.2384E7 | 274.8 | 247.3 | 98.0 |
| 1.3896E7 | 291.1 | 256.9 | 110.7 |
| 1.5588E7 | 304.2 | 264.7 | 120.9 |
| 1.7532E7 | 318.7 | 272.2 | 130.7 |
| 1.8216E7 | 324.5 | 273.5 | 133.6 |

Table 9: $g_i(t)$ for the linear with $N = 800$.

| $N$ | $\tau_D/10^5\ \tau$ | $t_{\boldsymbol{cc}}/\tau$ | $t_{R_g^2 R_g^2}/\tau$ |
|---|---|---|---|
| 100 | 0.07 | 4000 | 4200 |
| 200 | 0.39 | 11000 | 15000 |
| 400 | 2.38 | 45500 | 100000 |
| 800 | 20.0 | 273300 | 670000 |
| 1600 | $> 105.5$ | 1096000 | – |

Table 10: Data used in Fig. 5 of the article for the rings. The diffusion time is $\tau_D$, $t_{\boldsymbol{cc}}$ is the correlation time of the cross product of the spanning vectors and $t_{R_g^2 R_g^2}$ is the correlation time of the radius of gyration squared.
